# Supplementary material for: EMMOE: A Comprehensive Benchmark for Embodied Mobile Manipulation in Open Environments
Source: arXiv:2503.08604 source file (2025-05-15)
Supplement: Supplementary file 1 [file limitation.tex]

\section{Limitations and Future Works}
\label{sec:supp_limitation}

\paragraph{Limitations}
As we collect our dataset on Habitat HAB~\cite{szot2021habitat}, we also inherit some limitations of the simulator. Firstly, the range of available actions and interactive objects is limited, restricting the scope of our task design. Secondly, the environment is confined to a single-room setting, which does not effectively showcase the exploration process. When the scenario is expanded to multiple rooms, the demands on navigation and memory functions will significantly increase, potentially necessitating the integration of additional memory mechanisms. Besides, standardized outputs have increased the number of model inferences, which will bring additional time costs. Therefore, designing a more efficient workflow and output format is necessary.

\paragraph{Future works} 
Recently, more powerful simulators like Robocasa~\cite{nasiriany2024robocasa} have emerged, featuring more advanced skill primitives and interactive objects, enabling the design and collection of a wider range of everyday tasks. Additionally, since the simulator is used only for collecting image and video data, and evaluation metrics are not dependent on the simulator either, thus making real-world deployment of Homie possible. Furthermore, a home robot must be capable of interacting with family members, so exploring how Homie can interact or collaborate with humans to complete tasks is also worthful.
